# Supplementary material for: Mechanism, measurement, and quantification of stress in decision process: a model based systematic-review protocol
Source: arXiv:2203.10397 source file (2022-03-19)
Supplement: Supplementary file 2 [file Additional_file_3_SU.pdf]

# Search strategy

We will set no search limits on study design and type of intervention. The search strategy will focus on four key elements: definition (for example, psychological stress, workload), measurement (for example, EEG, HRV), quantification (for example, quantify, algorithm), and application (for example, training, driving). The definition of stress and its related concepts will be searched from significant articles and research. Considering the published time of these articles, regarding the definition of stress and stress-related concepts, may earlier than the searching range we original planned, the definition part will not be systematically reviewed. By considering the combination of measurement and quantification in stress experiment, the measurement and quantification of stress and its related concepts will be searched together. Then, we will search the application of stress and its related concepts.

Table 1. Search strategy for the keywords and search terms

| **Search terms** | **Keywords** |
| --- | --- |
| 1. Measurement and quantification | (“mental stress” OR “acute stress” OR “psychological stress” OR workload OR “cognitive workload” OR “cognitive engagement” OR affect OR fatigue) AND (EEG OR electroencephalogram OR “heart rate variability” OR HRV OR cortisol OR “electrodermal activity” OR EDA OR “galvanic skin response” OR “electrodermal assessment” OR “facial expression” OR “face reader” OR “facial expression analysis” OR “eye tracking” OR “NASA TLX” OR “NASA task load index”) OR (device OR protocol OR measurement OR experiment OR test OR measure OR equipment) OR (quantification OR quantify OR algorithm) AND (application OR design OR learning OR training OR driving OR HCI OR “human-computer interaction” OR ergonomics) |

| | |
|---|---|
| 2. Application | (application OR design OR learning OR training OR driving OR HCI OR “human-computer interaction” OR ergonomics) |
| 3. Publication time limit | Time range: 1990-2020 |
| 4. Participants | Limit: Adults: 19+ years |

Searches combined with AND: 1 AND 2 AND 3 AND 4.

Table 1 lists the search strategy. Subsequently, the Boolean operator "OR" will be merged to include synonyms and alternate spellings, and then the Boolean operator "AND" will be used to link the keywords and create the final search string.

## References


[1] B. Kitchenham and S. Charters, *Guidelines for performing Systematic Literature Reviews in Software Engineering*. 2007.
